# Supplementary material for: Reducing Degeneracy in Maximum Entropy Models of Networks
Source: arXiv:1407.0991 ancillary file (2015-03-17)
Supplement: Supplementary file 1 [file SupplMat.pdf]

## Animations

The animations can be played back by opening the files with any web browser.

- `ts_log_N.gif` shows $\ln \mathcal{N}(m_{|}, m_{\vee})$ as a 3D plot for graphs on 9 vertices.
- `tri_log_N.gif` shows $\ln \mathcal{N}(m_{|}, m_{\triangle})$ as a 3D plot for graphs on 9 vertices.
- `edges_ts_ani.gif` shows the distribution $p(m_{|}, m_{\vee})$ in the model ERG$(m_{|}, m_{\vee})$. The black dot shows the average $(\langle m_{|}\rangle, \langle m_{\vee}\rangle)$. As this point moves around, the distribution changes accordingly. For certain parameters it becomes bimodal (degenerate).
- `edges-squared_ts_ani.gif` The green dot shows $(\sqrt{\langle \boldsymbol{\xi}_{|}\rangle}, \langle \boldsymbol{\xi}_{\vee}\rangle) = (\sqrt{\langle m_{|}^2\rangle}, \langle m_{\vee}\rangle)$. The black dot shows $(\langle m_{|}\rangle, \langle m_{\vee}\rangle)$. The distribution is unimodal (non-degenerate) for all parameter values shown here. Correspondingly, these two averages (the black and green dots) are close to each other.

## Proof of the theorem for arbitrary dimensions

It follows the same steps as described in the main article for the 1D case. An ERG$(\mathbf{m})$ model is degenerate if there exists a $\boldsymbol{\beta}$ parameter value for which the sampled graphs differ significantly in at least one of the $m_i$ coordinates with high probability, for example, as in the case of a bimodal (or multimodal) $p(\mathbf{m}; \boldsymbol{\beta})$ with high peaks, whose separation is $\mathcal{O}(1)$, as discused above in the main paper. Below we provide the proof of our theorem for arbitrary dimensions.

**Proof:** We first make the observation that in two and higher dimensions degeneracy may still occur if we only demand that the distribution $p(\mathbf{m}; \boldsymbol{\beta})$ is unimodal. This is because unimodality alone is only a necessary condition for avoiding degeneracy, but not sufficient. An example is the “skewed hat” distribution of Fig. S1, which has only a single local maximum, but it is still degenerate (points from the rim of the “crater” are $\mathcal{O}(1)$ apart and are generated with high probability). Notice, however, that this distribution also has a local minimum and saddle point. The precise condition for non-degeneracy is that *all the stationary points* of the distribution be *local maxima*. Clearly, if the domain of the distribution is compact then we’ll only have one such maximum, which will also be the global maximum. Recall that throughout this proof we work with continuous, smoothened versions of the functions/distributions over continuous domains, and all functions are twice differentiable.

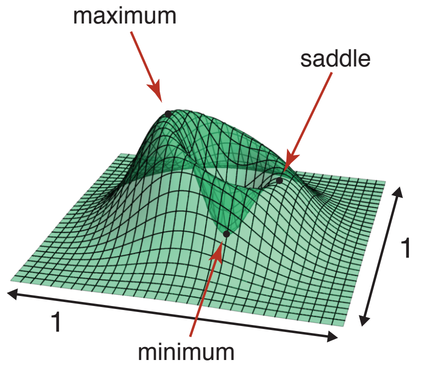


Figure S1: A “skewed hat” distribution is degenerate despite having a single local maximum. It has only one local maximum, but also a local minimum and a saddle point.

Let us consider the following function $g$,

$$g : \Omega \to \mathbb{R},$$
$$g(\mathbf{x}) = g(x_1, \ldots, x_N) = f(x_1, \ldots, x_N) e^{-(\beta_1 x_1 + \cdots + \beta_N x_N)} = f(\mathbf{x}) e^{-\boldsymbol{\beta}\cdot\mathbf{x}}, \tag{S1}$$

with

$$f : \Omega \to \mathbb{R}^+, \quad \text{that is,} \quad f(\mathbf{x}) > 0,\ \forall \mathbf{x} \in \Omega \subset \mathbb{R}^N$$

Here $f$ is the analog of $\mathcal{N}(\mathbf{m})$ and $g$ is the analog of $p(\mathbf{m}; \boldsymbol{\beta})$. $\Omega$ is the analog of $\mathcal{D}$, that is the domain where $\mathcal{N}(\mathbf{m}) > 0$, i.e., there exist graphs there with properties $\mathbf{m}$.

By definition, $\mathbf{x}^{(0)}$ is a stationary point of $g(\mathbf{x})$ if

$$\nabla g(\mathbf{x}^{(0)}) = 0 \quad \Leftrightarrow \quad \left.\frac{\partial g}{\partial x_i}\right|_{\mathbf{x}=\mathbf{x}^{(0)}} = 0,\ \forall i = 1, \ldots, N$$

From (S1):

$$\frac{\partial g}{\partial x_i} = \left(\frac{\partial f}{\partial x_i} - f\beta_i\right) e^{-\boldsymbol{\beta}\cdot\mathbf{x}}.$$

Thus, in a stationary point $\mathbf{x}^{(0)}$ of $g$:

$$\left.\frac{\partial f}{\partial x_i}\right|_{\mathbf{x}=\mathbf{x}^{(0)}} = f(\mathbf{x}^{(0)})\beta_i, \quad \forall i = 1, \ldots, N \tag{S2}$$

Combining for all $i$ we obtain the condition

$$\nabla f(\mathbf{x}^{(0)}) - f(\mathbf{x}^{(0)})\boldsymbol{\beta} = 0 \quad \Leftrightarrow \quad \boldsymbol{\beta} = \frac{\nabla f(\mathbf{x}^{(0)})}{f(\mathbf{x}^{(0)})} \tag{S3}$$

for $\mathbf{x}^{(0)}$ to be a stationary point of $g(\mathbf{x})$. Note that since $f(\mathbf{x}) \neq 0,\ \forall \mathbf{x} \in \Omega$, *any point* $\mathbf{x} = \mathbf{x}^{(0)} \in \Omega$ can become a stationary point of $g(\mathbf{x})$ by setting $\boldsymbol{\beta}$ to the value given in (S3).

Let us now demand that for a given $g$ (fixed $\boldsymbol{\beta}$) all the stationary points of $g$ are local *maxima*, thus ruling out any minima or saddle points. This is equivalent to demanding that the Hessian matrix with components

$$H_{ij} = \frac{\partial^2 g}{\partial x_i \partial x_j}$$

is negative semi-definite in all the stationary points. The components of the Hessian of $g$ can be written in terms of $f$ as

$$H_{ij} = \frac{\partial^2 g}{\partial x_i \partial x_j} = \left(\frac{\partial^2 f}{\partial x_i \partial x_j} - \frac{\partial f}{\partial x_j}\beta_i - \frac{\partial f}{\partial x_i}\beta_j + f\beta_i\beta_j\right) e^{-\boldsymbol{\beta}\cdot\mathbf{x}}.$$

The term $e^{-\boldsymbol{\beta}\cdot\mathbf{x}}$ is always positive, so asking that $H$ be negative semidefinite is equivalent to asking that the matrix $He^{\boldsymbol{\beta}\cdot\mathbf{x}}$ be negative semidefinite. Using (S2) we find that in a stationary point $\mathbf{x}^{(0)}$ the components of $He^{\boldsymbol{\beta}\cdot\mathbf{x}^{(0)}}$ are

$$[He^{\boldsymbol{\beta}\cdot\mathbf{x}^{(0)}}]_{ij} = \left.\frac{\partial^2 f}{\partial x_i \partial x_j}\right|_{\mathbf{x}=\mathbf{x}^{(0)}} - f(\mathbf{x}^{(0)})\beta_i\beta_j \tag{S4}$$

and therefore, the matrix $He^{\boldsymbol{\beta}\cdot\mathbf{x}}$ is negative semidefinite in the stationary point if and only if the rhs of (S4) is also negative semidefinite in the same point.

Let us now write down the components of the Hessian matrix of $\ln f$:

$$\frac{\partial^2 \ln f}{\partial x_i \partial x_j} = \frac{\partial}{\partial x_j}\left(\frac{1}{f(\mathbf{x})}\frac{\partial f}{\partial x_i}\right) = \frac{1}{f(\mathbf{x})}\frac{\partial^2 f}{\partial x_i \partial x_j} - \frac{1}{f(\mathbf{x})^2}\frac{\partial f}{\partial x_i}\frac{\partial f}{\partial x_j}$$

Thus in a stationary point (after using (S2)):

$$\Rightarrow \left.\frac{\partial^2 \ln f}{\partial x_i \partial x_j}\right|_{\mathbf{x}=\mathbf{x}^{(0)}} = \frac{1}{f(\mathbf{x}^{(0)})}\left[\left.\frac{\partial^2 f}{\partial x_i \partial x_j}\right|_{\mathbf{x}=\mathbf{x}^{(0)}} - f(\mathbf{x}^{(0)})\beta_i\beta_j\right] \stackrel{S4}{=} \frac{1}{f(\mathbf{x}^{(0)})}\left[He^{\boldsymbol{\beta}\cdot\mathbf{x}^{(0)}}\right]_{ij}. \quad \text{(S5)}$$

It is known that a multivariate function is concave if and only if its Hessian matrix is negative semi-definite. Thus (S5) establishes that the matrix $He^{\boldsymbol{\beta}\cdot\mathbf{x}}$ is negative semidefinite in a stationary point of $g$ if and only if $\ln f$ is concave in the same point (the $1/f > 0$ factor on the rhs does not affect this statement), or that $f$ is log-concave there. Since, as we have shown above, any point $\mathbf{x} \in \Omega$ can be made into a stationary point (there is a corresponding $\boldsymbol{\beta}$ parameter value), this implies that in order for an ERG($\mathbf{m}$) model not to be degenerate, $\mathcal{N}(\mathbf{m})$ has to be log-concave in all $\mathbf{x} \in \mathcal{D}$.

## Other examples

**1.** This example is from combinatorics/group theory. Since every finite group is isomorphic to a subgroup of the group of permutations, statements about permutations are applicable to finite groups [1]. Let the "microstates" be permutations of order $N$, so our state space is now the set of

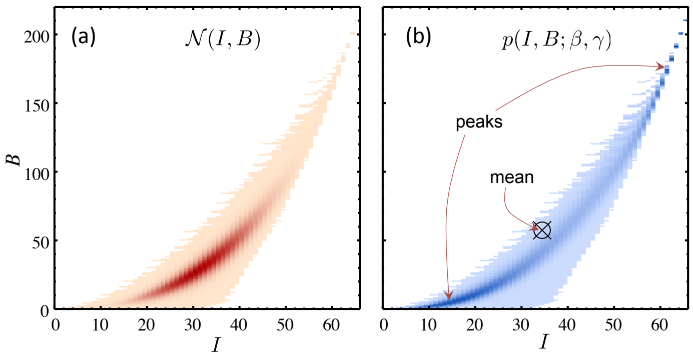


Figure S2: (a) $\mathcal{N}(I,B)$ for the set of permutations of order 10, where $I$ is the number of inversions and $B$ is the number of three-patterns that are out-of-order. (b) The distribution $p(I,B;\beta,\gamma)$ is bimodal for $\beta = 0.425$ and $\gamma = -0.1505$.

permutations of $N$ elements. Let $I$ be the number of inversions. An inversion is an out-of-order pair, e.g., in the permutation $a_1a_2\ldots a_N$, $a_ia_j$ is an inversion if $i < j$ but $a_i > a_j$. Let $B$ be the number of (for example) out-of-order 3-patterns [2], i.e., the number of triples $a_ia_ja_k$ where $i < j < k$ and it is *not* true that $a_i < a_j < a_k$. Since this is not an exponential random graph (ERG) model, the corresponding maximum entropy model will be denoted by MaxEnt. The MaxEnt($I,B$) model is degenerate because the domain of $\mathcal{N}(I,B)$ is not convex, and thus

$\mathcal{N}(I, B)$ is not a log-concave function, as shown in Fig. S2(a). Accordingly, the distribution $p(I, B; \beta, \gamma)$ is bimodal as shown in Fig. S2(b). An interesting paper is Ref [3] which uses a maximum entropy based modeling approach to predict permutations as outcomes in horse races.

**2.** Here we demonstrate fitting an ERG model to another network, a larger graph of 198 nodes that describes a collaboration network of jazz musicians [4]. In addition, we also work with a three-variable model instead of two variables.

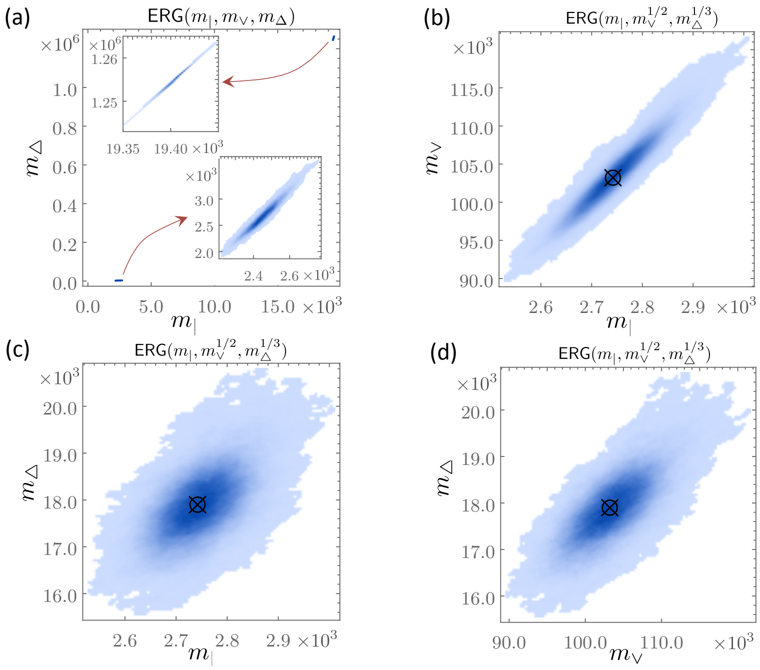


Figure S3: (a) Trying to fit the jazz musicians network with 198 nodes shows degeneracy. Notice the wide separation of the high probability peaks in $p(\mathbf{m}; \boldsymbol{\beta})$. The distributions $p(m_|, m_\vee; \boldsymbol{\beta})$, $p(m_|, m_\Delta; \boldsymbol{\beta})$ and $p(m_\vee, m_\Delta; \boldsymbol{\beta})$ obtained after fitting ERG($m_|, m_\vee^{1/2}, m_\Delta^{1/3}$), which is not degenerate. The fitting parameters are $\beta_| = 1.82$, $\beta_\vee = 12.5$ and $\beta_\Delta = -313$.

This network has $m_|^0 = 2742$ edges, $m_\vee^0 = 103\,212$ two-stars and $m_\Delta^0 = 17\,899$ triangles. When trying to fit ERG($m_|, m_\Delta, m_\vee$) to these values, we run into the degeneracy problem as illustrated in Fig S3(a). Recall that degeneracy implies there are parameter values for which the $p(\mathbf{m}; \boldsymbol{\beta})$ distribution has significant masses in regions that are separated by large distances along at least one coordinate, as shown in Fig S3(a). The MCMC sampler once enters one of the regions, it will only leave it after extremely long times and which regions it gets trapped in depends on the initial conditions. We were not able to get converging parameter values for the duration of the simulations which were run for several days. However, using the transformed quantities as proposed in the paper and fitting ERG($m_|, m_\vee^{1/2}, m_\Delta^{1/3}$), it eliminates these problems and fitting is feasible computationally as well. The non-degenerate distributions in all the three projections after the fitting are shown in Fig. S3(b-d). The crosses indicate the locations of the

mean values. Indeed, the sampling probability is concentrated around the means, along all the coordinates.

# References


[1] P. Ramond. *Group Theory: A Physicist's Survey* (Cambridge University Press, 2010).

[2] M. Bóna. *Combinatorics of Permutations (Discrete Mathematics and its Applications)*. (Chapman & Hall/CRC Press, 2004).

[3] S. Agrawal, Z. Z. Wang, Y. Y. Ye, Parimutuel Betting on Permutations. Internet and Network Economics, *Proceedings, Lecture Notes in Computer Science*, **5385**, 126-137 (2008).

[4] P. Gleiser and L. Danon, Community structure in jazz. *Adv. Complex Syst.* **6**, 565-573 (2003).
